# Supplementary material for: Optimizing over Serial Dictatorships
Source: arXiv:2202.08097 source file (2022-09-08)
Supplement: Supplementary file 1 [file additional-results.tex]

\subsection{Longest paths}

In this section, we explore the instances of 
$\pro$ when valuations are derived from a 
complete directed graph $G$ with vertex set $[n]$, and weights $w(i \rightarrow j)$ for directed edges $i \rightarrow j$ with $i,j \in [n]$. \emph{Longest paths} in $G$ are defined as a union of (directed) disjoint paths where each node has at most one out-degree and at most one in-degree.
Given a weighted directed graph $G$, the problem is to find longest paths with maximum possible weight in $G$. We will refer the above optimization problem as $\paths$. 

Note that, in the query model of $\pro$, an algorithm can access the weights in the underlying graph $G$ via action sequences, i.e., it does not have direct access to the weights in $G$. For a node $i \in [n]$ and an ordered sequence $S$ of a subset of the remaining $n-1$ agents, we define the valuation query $v_i(S)$ as the maximum weight of a directed edge $(i \rightarrow j)$ such that its addition to the set of edges chosen by agents in $S$ is a union of paths in $G$. In particular, we have $v_i(\phi) = \max_{j \neq i} w(i \rightarrow j)$, and we call the corresponding edge as \emph{top-choice} edge of node $i$ in $G$. It is trivial to observe that for any ordered subset $S'$ of $S$, we have $v_i(S') \geq v_i(S)$, i.e., $v_i$s are monotone.

For a given instance of $\paths$ in the above query model, the goal is to find an action sequence $\pi  \in S_n$ that maximizes the sum of valuations of all agents, $\sum_{i \in [n]} v_i(\pi^i)$.
We prove that the price of serial dictatorship (PoSD) for $\paths$ is strictly greater than one (Theorem~\ref{theorem: paths SD}).

\begin{theorem} \label{theorem: paths SD}
	An optimal solution for instances of $\textsc{Longest-Paths}$ may not be produced by any action sequence of nodes. Moreover, the price of serial dictatorship for $\paths$ is at least $3/2$.
\end{theorem}

\begin{proof}
	We construct an instance of $\textsc{Longest-Paths}$ consisting of four nodes $x_1, x_2, x_3$ and $x_4$ with following weights: $w(x_1 \rightarrow x_2) = w(x_2 \rightarrow x_3) =  w(x_3 \rightarrow x_4) = 1$; and $w(x_1 \rightarrow x_4) = w(x_2 \rightarrow x_4) = w(x_3 \rightarrow x_2) = 1+\varepsilon$. All the remaining edges have zero weight. Here, the unique optimal solution is the path $x_1 \rightarrow x_2 \rightarrow x_3 \rightarrow x_4$ having a weight of $3$, whereas any action sequence of these four nodes can achieve a value of at most $2+\varepsilon$. The price of serial dictatorship for $\textsc{Longest-Paths}$ is therefore at most $2/3$.
\end{proof}

The above lemma holds true for the problem of finding a Hamiltonian path of maximum weight.

%\section{Fairness with respect to Serial Dictatorship}

%\subsection{Maximum Cuts}

%\begin{lemma}
%There exists an algorithm that produces a $2$-approximation for a given instance of MAX-CUT using polynomially-many queries.
%\end{lemma}
